# Supplementary material for: Atomic resolution mapping of phonon excitations in STEM-EELS experiments
Source: arXiv:1403.1849 source file (2014-03-06)
Supplement: Supplementary file 1 [file Supplementalmaterial_Ricardo_Egoavil.pdf]

# Supplementary information: Atomic resolution mapping of phonon excitations in STEM-EELS experiments

R. Egoavil<sup>a</sup>, N. Gauquelin<sup>a</sup>, G. T. Martinez<sup>a</sup>, S. Van Aert<sup>a</sup>, G. Van Tendeloo<sup>a</sup>,  
J. Verbeeck<sup>a</sup>

<sup>a</sup>*EMAT, University of Antwerp, Department of Physics  
Groenenborgerlaan 171, B-2020 Antwerp, Belgium*

---

---

## 1. Supplementary material

Preservation of elastic contrast is unavoidable. In order to understand more about the significance of this atomic scale variation of the ZLP, one can integrate the normalised low loss signal in the following energy ranges [-1.0 to -0.5 eV]; [-0.5 eV to -0.14 eV]; [-0.14 to 0.14 eV]; [0.14 to 0.5 eV]; [1.0 to 3.2 eV]; [3.2 to 8.0 eV] and [8.0 to 15 eV] as presented on Figure 1. The results are in excellent agreement with S. Lazar [1], showing complementary contrast to the HAADF signal in the [-0.14 to 0.14 eV] energy region. Furthermore, clear positive atomically resolved signatures are observed in the energy ranges of [-1.0 to -0.5 eV]; [-0.5 eV to -0.14 eV] and [0.14 to 0.5 eV]. Clear attenuation of the contrast is observed close to the ZLP in the range of [1.0 to 3.2 eV], below the bandgap region for SrTiO<sub>3</sub>. Regions [3.2 to 8.0 eV] and [8.0 to 15 eV] show the absence of atomic contrast on the spectral range corresponding to the interband and plasmon energy losses respectively in good agreement with the expected delocalisation limits for electronic excitations.

---

\*Corresponding author

Email address: `ricardo.egoavil@uantwerpen.ua.ac.be` (R. Egoavil)

## 2. Results obtained at 300kV

A monocrystalline substrate of  $\text{SrTiO}_3$  with  $\sim 18\text{-}20$  nm thickness was investigated using a TEM lamella prepared perpendicular to the  $[100]$  zone axis orientation by focused ion beam milling. HAADF imaging, Scanning transmission electron microscopy (STEM) and EELS experiments were performed using the QuAntEM microscope at the University of Antwerp. This is an FEI Titan<sup>3</sup> microscope, equipped with an aberration corrector for both image and probe forming lenses, and a monochromator to optimize the energy resolution for EELS measurements up to 300 meV, as determined from the full width at half maximum (FWHM) of the ZLP. We performed experiments at an acceleration voltage of 300 keV where spatial resolution performance is approx.  $\sim 1.2(3)$  Å (probe size) at a convergence semi-angle of 21 mrad. The collection semi-angle  $\beta$  of the spectrometer was set to  $\sim 129$  mrad.

Figures 2 show the results obtained at 300 keV and  $\beta = 129$  mrad. The average unit cell HAADF image and its corresponding *divided* and *subtracted* 2D maps and spectra profiles in the range of energy -1 to 1 eV are presented. The broadening and shrinking of the ZLP is observed when comparing the 3 different Sr, TiO and O atomic columns, respectively, similar to the results obtained at 120 kV presented in the main text. Some deviation from the averaged spectrum extending to 1.5 eV on each side of the ZLP can be noticed.

## References

### 3. Supplementary information

## References

- [1] S. Lazar, Y. Shao, L. Gunawan, R. Nechache, A. Pignolet, G. A. Botton, Imaging, core-loss, and low-loss electron-energy-loss spectroscopy mapping in aberration-corrected STEM, *Microscopy and Microanalysis* 16 (04) (2010) 416–424.

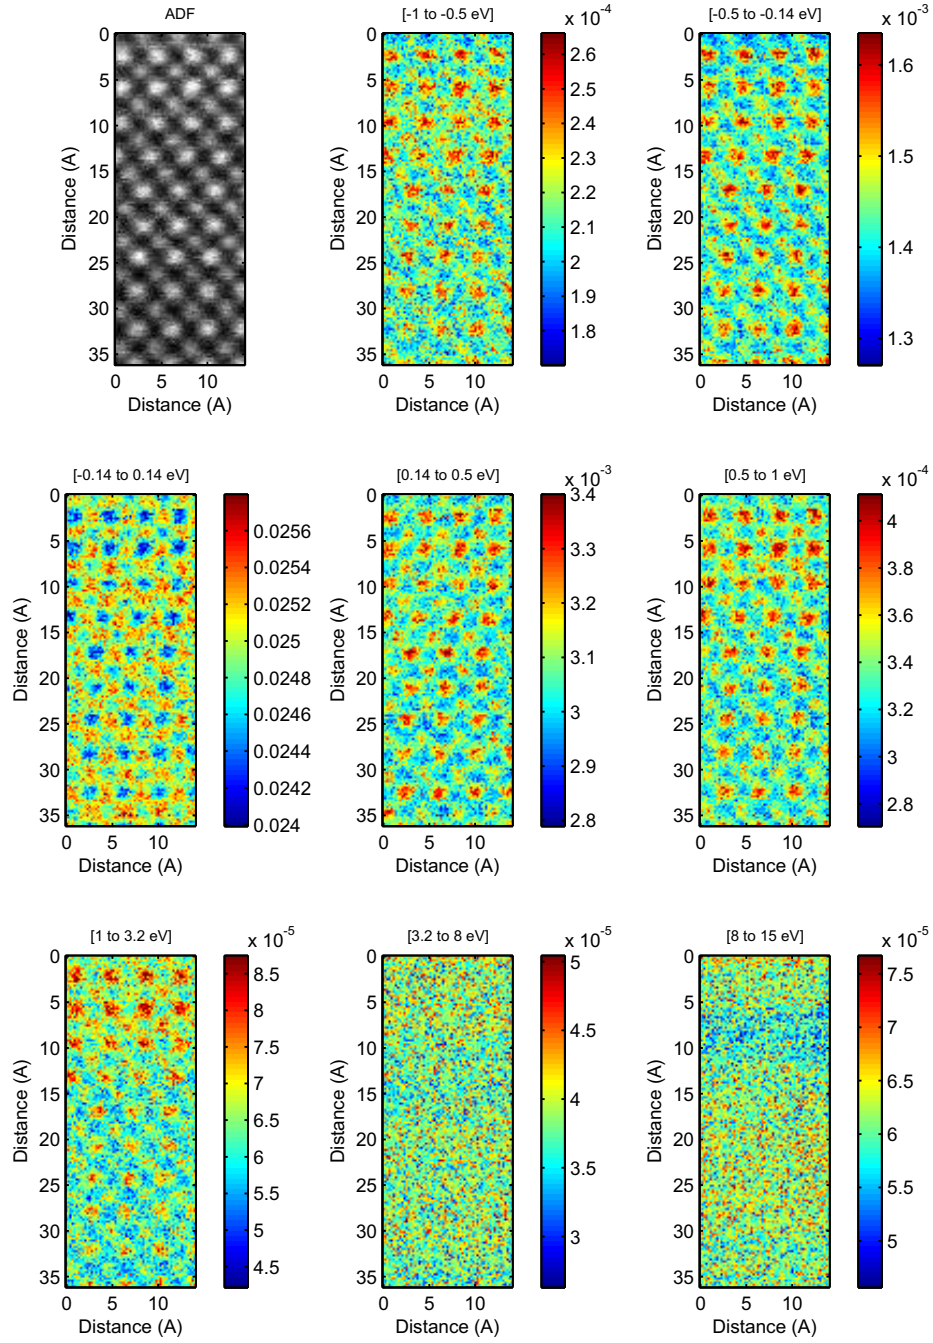

Figure 1: ADF image acquired at 120kV and its corresponding selected low loss signal integrated over different energy ranges of  $[-1.0$  to  $-0.5$  eV];  $[-0.5$  eV to  $-0.14$  eV];  $[-0.14$  to  $0.14$  eV];  $[0.14$  to  $0.5$  eV];  $[1.0$  to  $3.2$  eV];  $[3.2$  to  $8.0$  eV] and  $[8.0$  to  $15$  eV].

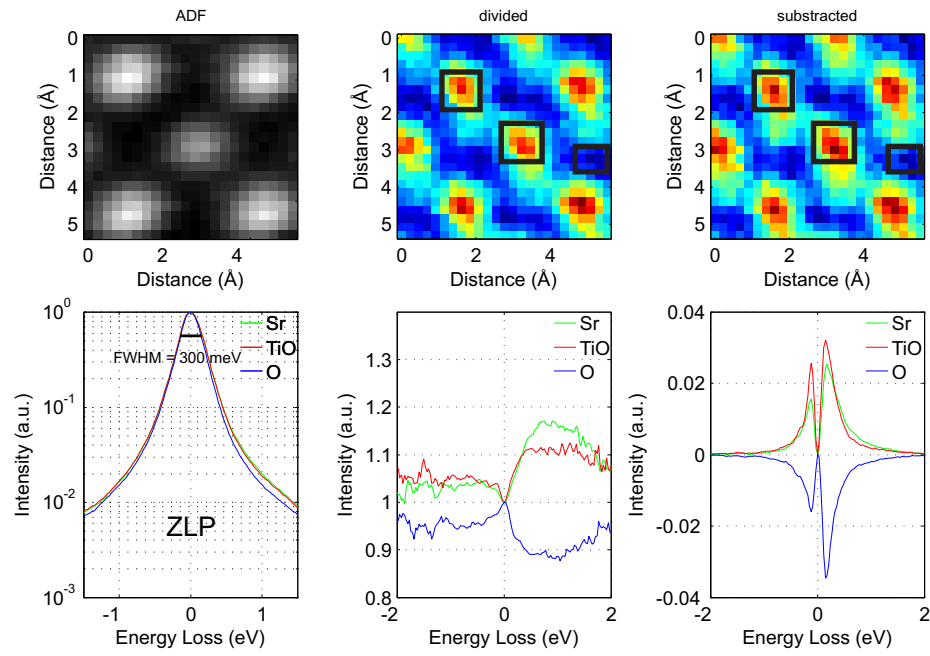

Figure 2: Averaged unit cell ADF image acquired at 300 kV, showing the *divided* and *subtracted* EELS maps and its corresponding integrated spectra profiles after averaging over 16 unit cells.
